# Supplementary material for: Quantum Fluctuations of the Stress-Energy Tensor via Noether's Theorem and the Connection to the Cosmological Constant
Source: arXiv:2611.14875 source file (2026-11-11)
Supplement: Supplementary file 1 [file Supplementary_Information.tex]

\documentclass[onecolumn,superscriptaddress,pra]{revtex4}
\usepackage{amsmath}
\usepackage{amssymb}
\usepackage{graphicx}
\usepackage{bm}

\begin{document}

\title{Supplementary Information: Quantum Fluctuations of the Stress-Energy Tensor via Noether's Theorem.}

\author{J. A. Crosse}
\email{jac32@nyu.edu}
\affiliation{New York University Shanghai, 1555 Century Avenue, Pudong, Shanghai, 200122, China.}
\affiliation{NYU-ECNU Institute of Physics at NYU Shanghai, 3663 Zhongshan Road North, Shanghai, 200062, China.}

\maketitle

\section{Lagrangian Field Theory}

\subsection{Euler-Lagrange Equation}

The action, $S$, is defined as the time integral over the Lagrangian, $L$, or equivalently the space-time integral over the Lagrangian density, $\mathcal{L}$,
\begin{equation}
S = \int dt\, L = \int d^{4}x\,\mathcal{L}.
\end{equation}
Both the Lagrangian, $L$, and the Lagrangian density, $\mathcal{L}$, are functions of the field, $\phi$, and its derivatives, $\partial_{\mu}\phi$. The principle of stationary action states that a system will evolve such that the action is minimized, i.e. $\delta S = 0$. Varying the action leads to
\begin{align}
\delta S &= \delta\int d^{4}x\,\mathcal{L},\nonumber\\
&= \int d^{4}x\,\left\{\frac{\partial \mathcal{L}}{\partial \phi}\delta\phi + \frac{\partial \mathcal{L}}{\partial (\partial_{\mu}\phi)}\delta(\partial_{\mu}\phi)\right\},\nonumber\\
&= \int d^{4}x\,\left\{\frac{\partial \mathcal{L}}{\partial \phi}\delta\phi + \frac{\partial \mathcal{L}}{\partial (\partial_{\mu}\phi)}\partial_{\mu}\delta\phi\right\},\nonumber\\
&= \int d^{4}x\,\left\{\frac{\partial \mathcal{L}}{\partial \phi}\delta\phi - \partial_{\mu}\left(\frac{\partial \mathcal{L}}{\partial (\partial_{\mu}\phi)}\right)\delta\phi+\partial_{\mu}\left(\frac{\partial \mathcal{L}}{\partial (\partial_{\mu}\phi)}\delta\phi\right)\right\},
\end{align}
where in the last line we have applied the product rule of differentiation. The last term is a divergence. By Gauss' Law this becomes an integral of that quantity over the surface of the volume. As the field is fixed at the surface of the volume by the boundary conditions we impose, $\delta\phi=0$ on the surface. Thus, the last term vanishes and one obtains
\begin{align}
\delta S &= \int d^{4}x\,\left\{\frac{\partial \mathcal{L}}{\partial \phi}\delta\phi - \partial_{\mu}\left(\frac{\partial \mathcal{L}}{\partial (\partial_{\mu}\phi)}\right)\delta\phi\right\},\nonumber\\
&= \int d^{4}x\,\left\{\frac{\partial \mathcal{L}}{\partial \phi} - \partial_{\mu}\left(\frac{\partial \mathcal{L}}{\partial (\partial_{\mu}\phi)}\right)\right\}\delta\phi.
\end{align}
Within the volume $\delta\phi \neq 0$ and, hence, for $\delta S$ to vanish for all values of $\delta\phi$ then one must have
\begin{equation}
\frac{\partial \mathcal{L}}{\partial \phi} - \partial_{\mu}\left(\frac{\partial \mathcal{L}}{\partial (\partial_{\mu}\phi)}\right) = 0.
\end{equation}
This is the Euler-Lagrange Equation, the equation of motion for the field, $\phi$, that defines the classical path along which the field will evolve.

\subsection{Noether's Theorem}

Noether's Theorem states that if the action, $S$, is invariant under some transformation then there is an associated conserved quantity. Thus, if we vary the field
\begin{equation}
\phi \rightarrow \phi' = \phi + \alpha\delta\phi,
\label{phivary}
\end{equation}
and the action, $S$, or equivalently the Lagrangian density, $\mathcal{L}$, is unchanged up to a divergence (surface term)
\begin{equation}
\mathcal{L}(\phi) \rightarrow \mathcal{L}'(\phi') = \mathcal{L}(\phi') - \alpha\partial_{\mu}J^{\mu},
\label{Lvary}
\end{equation}
then we can find some combinations of parameters that remains unchanged as the field evolves. We can find an expression for this conserved quantity by varying action
\begin{align}
\delta S &= \delta\int d^{4}x\,\mathcal{L}',\nonumber\\
&= \delta\int d^{4}x\,\left\{\mathcal{L} - \alpha\partial_{\mu}J^{\mu}\right\},\nonumber\\
&= \int d^{4}x\,\left\{\frac{\partial \mathcal{L}}{\partial \phi}\alpha\delta\phi + \frac{\partial \mathcal{L}}{\partial (\partial_{\mu}\phi)}\delta(\alpha\partial_{\mu}\phi)-\alpha\partial_{\mu}J^{\mu}\right\}.
\end{align}
Applying the product rule gives
\begin{align}
\delta S &= \int d^{4}x\,\left\{\frac{\partial \mathcal{L}}{\partial \phi}\alpha\delta\phi + \frac{\partial \mathcal{L}}{\partial (\partial_{\mu}\phi)}\partial_{\mu}(\alpha\delta\phi)-\alpha\partial_{\mu}J^{\mu}\right\},\nonumber\\
&= \int d^{4}x\,\left\{\frac{\partial \mathcal{L}}{\partial \phi}\alpha\delta\phi - \partial_{\mu}\left(\frac{\partial \mathcal{L}}{\partial (\partial_{\mu}\phi)}\right)\alpha\delta\phi+\partial_{\mu}\left(\frac{\partial \mathcal{L}}{\partial (\partial_{\mu}\phi)}\alpha\delta\phi\right)-\alpha\partial_{\mu}J^{\mu}\right\},\nonumber\\
&=\alpha\int d^{4}x\,\partial_{\mu}\left\{\left(\frac{\partial \mathcal{L}}{\partial (\partial_{\mu}\phi)}\delta\phi\right)-J^{\mu}\right\} +  \alpha\int d^{4}x\,\left\{\frac{\partial \mathcal{L}}{\partial \phi} - \partial_{\mu}\left(\frac{\partial \mathcal{L}}{\partial (\partial_{\mu}\phi)}\right)\right\}\delta\phi.
\label{noether}
\end{align}
The second term vanishes because the integrand is just the Euler-Lagrange equation which is identically zero along the classical path. For the action, $S$, to be unchanged by the variation the first term must also vanish
\begin{equation}
\alpha\int d^{4}x\,\partial_{\mu}\left\{\left(\frac{\partial \mathcal{L}}{\partial (\partial_{\mu}\phi)}\delta\phi\right)-J^{\mu}\right\} = 0,
\end{equation}
and, hence, the integrand must vanish
\begin{equation}
\partial_{\mu}\left\{\left(\frac{\partial \mathcal{L}}{\partial (\partial_{\mu}\phi)}\delta\phi\right)-J^{\mu}\right\} = 0,
\end{equation}
and, thus, the expression within the derivative must be a constant
\begin{equation}
j^{\mu} = \left(\frac{\partial \mathcal{L}}{\partial (\partial_{\mu}\phi)}\delta\phi\right)-J^{\mu}.
\end{equation}
This quantity, $ j^{\mu}$, is known as the Noether's Current and is a constant of motion.

\subsection{Stress-Energy Tensor}

As an example one can look at a spacetime transformation that leaves the action, $S$, unchanged
\begin{equation}
x^{\mu} \rightarrow x'^{\mu} = x^{\mu} + a^{\mu}.
\end{equation}
The field the becomes
\begin{equation}
\phi(x^{\mu}) \rightarrow \phi(x'^{\mu}) = \phi(x^{\mu} + a^{\mu}) = \phi(x^{\mu}) + a^{\mu}\partial_{\mu}\phi(x^{\mu}),
\label{phivary2}
\end{equation}
and the Lagrangian density becomes
\begin{equation}
\mathcal{L}(x^{\mu}) \rightarrow \mathcal{L}(x'^{\mu}) = \mathcal{L}(x^{\mu} + a^{\mu}) = \mathcal{L}(x^{\mu}) + a^{\mu}\partial_{\mu}\mathcal{L}(x^{\mu}).
\label{Lvary2}
\end{equation}
Comparing Eqs. \eqref{phivary} and \eqref{phivary2} gives the variation in the field
\begin{equation}
\alpha \delta \phi = a^{\mu}\partial_{\mu}\phi = a^{\nu}\partial_{\nu}\phi.
\end{equation}
Comparing Eqs. \eqref{Lvary} and \eqref{Lvary2} implies that
\begin{equation}
\alpha \partial_{\mu}J^{\mu} = a^{\mu}\partial_{\mu}\mathcal{L} = a^{\nu}\eta_{\;\;\nu}^{\mu}\partial_{\mu}\mathcal{L} = a^{\nu}\partial_{\mu}\left(\eta_{\;\;\nu}^{\mu}\mathcal{L}\right),\nonumber
\end{equation}
where $\eta_{\;\;\nu}^{\mu}$ is the flat space Minkowski metric. Hence, the conserved quantity is given by
\begin{equation}
T^{\mu}_{\;\;\nu} = \left(\frac{\partial \mathcal{L}}{\partial (\partial_{\mu}\phi)}\delta\phi\right)-J^{\mu} = \left(\frac{\partial \mathcal{L}}{\partial (\partial_{\mu}\phi)}\right)\partial_{\nu}\phi-\eta_{\;\;\nu}^{\mu}\mathcal{L},
\end{equation}
which is the Stress-Energy Tensor.

\section{Quantum Fluctuations of the Noether's Current}

\subsection{Conserved Current Fluctuations}

The above analysis assumes that the system follows the classical path. However, Feynman's path integral quantization formalism implies that quantum fields do not necessarily evolve this way. If the system does not follow the classical path, the first term in Eq. \eqref{noether} would not vanish as the evolution of the field would not be described by the Euler-Lagrange equation
\begin{equation}
\alpha\int d^{4}x\,\partial_{\mu}F^{\mu} = \alpha\int d^{4}x\,\left\{\frac{\partial \mathcal{L}}{\partial \phi} - \partial_{\mu}\left(\frac{\partial \mathcal{L}}{\partial (\partial_{\mu}\phi)}\right)\right\}\delta\phi \neq 0.
\label{f1}
\end{equation}
In this case, $F^{\mu}$ will also contribute to the conserved current and would be a fluctuation in the Noether's current owing to the field not evolving along the classical path
\begin{equation}
j^{\mu} = \left(\frac{\partial \mathcal{L}}{\partial (\partial_{\mu}\phi)}\delta\phi\right)-J^{\mu} + F^{\mu}.
\end{equation}
In order to compute $F^{\mu}$ one can functionally expand the action, $S$, about the field values that solve the Euler-Lagrange Equation (i.e. the classical path)
\begin{align}
S(\phi_{cl}+\Delta\phi) &= S_{0} + S_{1} + S_{2} + \cdots,\nonumber\\
&= S(\phi_{cl}) + \int d^{4}x' \,\Delta\phi(x')\left.\frac{\delta S}{\delta \phi(x')}\right|_{\phi_{cl}}\nonumber\\
&\hspace{3cm} + \frac{1}{2!}\int d^{4}x'\int d^{4}x''\, \Delta\phi(x')\Delta\phi(x'')\left.\frac{\delta^{2} S}{\delta \phi(x')\delta \phi(x'')}\right|_{\phi_{cl}} + \cdots.
\end{align}
The zeroth order term, $S_{0}$, is just the action along the classical path, which obeys the Euler-Lagrange Equation and so it's contribution to the fluctuations, $F^{\mu}$, vanishes. The first order term, $S_{1}$, is the variation of the action which, by definition, is equal to zero along the classical path. The lowest order term to contribute to the fluctuations is the second order term, $S_{2}$. We can rewrite the second order term, $S_2$, in terms of the Lagrangian density, $\mathcal{L}$, as
\begin{align}
S_2 &= \frac{1}{2!}\int d^{4}x'\int d^{4}x'' \,\Delta\phi(x')\Delta\phi(x'')\left.\frac{\delta^{2} S}{\delta \phi(x')\delta \phi(x'')}\right|_{\phi_{cl}} ,\nonumber\\
&= \frac{1}{2!}\int d^{4}x\int d^{4}x'\int d^{4}x''\, \Delta\phi(x')\Delta\phi(x'')\left.\frac{\delta^{2} \mathcal{L}}{\delta \phi(x')\delta \phi(x'')}\right|_{\phi_{cl}},\nonumber\\
&= \int d^{4}x\, \mathcal{L}_{2}.
\end{align}

\subsection{Fluctuations in the Stress-Energy Tensor}

If the Lagrangian density is bilinear or quadratic in the field or its derivative, then the second order functional derivatives will result in two times the constant prefactor for that term, which cancels the factor of half from the functional expansion. Hence, the effect of the expansion is to replace the field, $\phi(x)$, in the Lagrangian density with the deviation of the field form the classical value, $\Delta\phi(x)$,
\begin{equation}
\mathcal{L}_{2}\left[\phi(x),\partial_{\mu}\phi(x)\right] = \mathcal{L}\left[\Delta\phi(x),\partial_{\mu}\Delta\phi(x)\right].
\label{L2}
\end{equation}
Furthermore, this term will be the highest order term in the expansion. All higher order terms will vanish. 

One can compute the fluctuations, $F^{\mu}$, by substituting Eq. \eqref{L2} into Eq. \eqref{f1} and changing variables $\phi(x) \rightarrow \phi_{cl}(x) + \Delta\phi(x)$ where $\phi_{cl}(x)$ is the classical value of the field and acts as a constant. Thus,
\begin{align}
\alpha\int d^{4}x\,\partial_{\mu}F^{\mu} &= \alpha\int d^{4}x\,\left\{\frac{\partial \mathcal{L}_{2}\left[\phi\right]}{\partial \phi} - \partial_{\mu}\left(\frac{\partial \mathcal{L}_{2}\left[\phi\right]}{\partial (\partial_{\mu}\phi)}\right)\right\}\delta\phi,\nonumber\\
&= \alpha\int d^{4}x\,\left\{\frac{\partial \mathcal{L}\left[\Delta\phi\right]}{\partial \Delta\phi} - \partial_{\mu}\left(\frac{\partial \mathcal{L}\left[\Delta\phi\right]}{\partial (\partial_{\mu}\Delta\phi)}\right)\right\}\delta\Delta\phi.
\end{align}
One can simplify this by noting that 
\begin{equation}
\partial_{\nu}\mathcal{L} = \frac{\partial\mathcal{L}}{\partial\Delta\phi}\partial_{\nu}\Delta\phi + \frac{\partial\mathcal{L}}{\partial(\partial_{\mu}\Delta\phi)}\partial_{\nu}\left(\partial_{\mu}\Delta\phi\right),
\end{equation}
and recalling that for a spacetime translation $\alpha \delta \Delta\phi =  a^{\nu}\partial_{\nu}\Delta\phi$, one finds
\begin{align}
\alpha\int d^{4}x\,\partial_{\mu}F^{\mu} &= a^{\nu}\int d^{4}x\,\left\{\frac{\partial \mathcal{L}\left[\Delta\phi\right]\left[\Delta\phi\right]}{\partial \Delta\phi}\partial_{\nu}\Delta\phi - \partial_{\mu}\left(\frac{\partial \mathcal{L}\left[\Delta\phi\right]\left[\Delta\phi\right]}{\partial (\partial_{\mu}\Delta\phi)}\right)\partial_{\nu}\Delta\phi\right\},\nonumber\\
&= a^{\nu}\int d^{4}x\,\left\{\partial_{\nu}\mathcal{L}\left[\Delta\phi\right] - \frac{\partial\mathcal{L}}{\partial(\partial_{\mu}\Delta\phi)}\partial_{\nu}\left(\partial_{\mu}\Delta\phi\right) - \partial_{\mu}\left(\frac{\partial \mathcal{L}\left[\Delta\phi\right]\left[\Delta\phi\right]}{\partial (\partial_{\mu}\Delta\phi)}\right)\partial_{\nu}\Delta\phi\right\},\nonumber\\
&= a^{\nu}\int d^{4}x\,\left\{\partial_{\mu}\eta_{\;\;\nu}^{\mu}\mathcal{L}\left[\Delta\phi\right] - \partial_{\mu}\left(\frac{\partial\mathcal{L}\left[\Delta\phi\right]}{\partial(\partial_{\mu}\Delta\phi)}\partial_{\nu}\Delta\phi\right)\right\},\nonumber\\
&= a^{\nu}\int d^{4}x\,\partial_{\mu}\left\{-\left(\frac{\partial\mathcal{L}\left[\Delta\phi\right]}{\partial(\partial_{\mu}\Delta\phi)}\partial_{\nu}\Delta\phi\right)+\eta_{\;\;\nu}^{\mu}\mathcal{L}\left[\Delta\phi\right]\right\}.
\label{f3}
\end{align}
The expression in the brackets is the Stress-Energy tensor except evaluated at the deviation of the field from the classical value, $\Delta\phi(x)$, rather than at the classical field value, $\phi(x)$, itself. Comparing the left and right hand sides of Eq. \eqref{f3} one can see the fluctuation, $F_{\;\;\nu}^{\mu}$, is given by
\begin{equation}
F_{\;\;\nu}^{\mu} = -\left\{\left(\frac{\partial\mathcal{L}\left[\Delta\phi\right]}{\partial(\partial_{\mu}\Delta\phi)}\partial_{\nu}\Delta\phi\right)-\eta_{\;\;\nu}^{\mu}\mathcal{L}\left[\Delta\phi\right]\right\} = -T^{\mu}_{\;\;\nu}(\Delta\phi),
\end{equation} 
which is minus the Stress-Energy tensor evaluated for the deviation of the field from the classical value.

\section{Example: Fluctuations in the Stress-Energy Tensor of a Free Complex Scalar Field}

\subsection{Fluctuations in a Free Complex Scalar Field}

As an example we can compute the Stress-Energy Tensor fluctuations of a free complex scalar field. The Lagrangian density, $\mathcal{L}$, for a complex scalar is given by
\begin{equation}
\mathcal{L}(\phi,\phi^\ast) = \partial_{\mu}\phi^\ast(x)\partial^{\mu}\phi(x) - m^2\phi^\ast(x)\phi(x),
\end{equation}
where $m$ is in units of $L^{-1}$. The conversion to mass in SI units, $\bar{m}$, is given by $m = \bar{m}c/\hbar$. Expanding the action about the classical field values, $\phi_{cl}$ and $\phi^\ast_{cl}$ gives
\begin{align}
S(\phi_{cl}+\Delta\phi, \phi^\ast_{cl}+\Delta\phi^\ast) = S(\phi_{cl}, \phi_{cl})  &+ \int d^{4}x' \,\Delta\phi^\ast(x')\left.\frac{\delta S}{\delta \phi^\ast(x')}\right|_{\phi^\ast_{cl}, \phi_{cl}}\nonumber\\
&\hspace{1cm} + \int d^{4}x'' \,\Delta\phi(x'')\left.\frac{\delta S}{\delta \phi(x'')}\right|_{\phi^\ast_{cl}, \phi_{cl}}\nonumber\\
&\hspace{2cm} + \int d^{4}x'\int d^{4}x''\, \Delta\phi^\ast(x')\Delta\phi(x'')\left.\frac{\delta^{2} S}{\delta \phi^\ast(x')\delta \phi(x'')}\right|_{\phi^\ast_{cl}, \phi_{cl}}.
\end{align}
Note that, as the action, $S$, is bilinear in the field, $\phi$, and the conjugate field, $\phi^\ast$, this expansion is exact. The functional derivatives of the action are 
\begin{align}
\left.\frac{\delta S}{\delta \phi^\ast(x')}\right|_{\phi_{cl}, \phi^\ast_{cl}} &= \int d^{4}x\,\left.\frac{\delta \mathcal{L}}{\delta \phi^\ast(x')}\right|_{\phi^\ast_{cl}, \phi_{cl}} ,\nonumber\\
&= \int d^{4}x\,\left.\left\{\partial_{\mu}\frac{\delta\phi^\ast(x)}{\delta \phi^\ast(x')}\partial^{\mu}\phi(x) - m^2\frac{\delta\phi^\ast(x)}{\delta\phi^\ast(x')}\phi(x)\right\}\right|_{\phi_{cl}, \phi^\ast_{cl}},\nonumber\\
&= \int d^{4}x\,\left.\left\{\partial_{\mu}\delta(x-x')\partial^{\mu}\phi(x) - m^2\delta(x-x')\phi(x)\right\}\right|_{\phi_{cl}, \phi^\ast_{cl}},\nonumber\\
&= \int d^{4}x\,\left.\left\{-\partial_{\mu}\partial^{\mu}\phi(x) - m^2\phi(x)\right\}\delta(x-x')\right|_{\phi_{cl}, \phi^\ast_{cl}}=0,
\end{align}
where in the last line we have used the fact that the expression in the brackets is the Klein-Gordon equation for the field, which vanishes for the classical field. This is expected as the first functional derivative vanishes at the minimum of the action, which is the definition of the classical path. Similarly
\begin{align}
\left.\frac{\delta S}{\delta \phi(x'')}\right|_{\phi_{cl}, \phi^\ast_{cl}} &= \int d^{4}x\,\left.\frac{\delta \mathcal{L}}{\delta \phi(x'')}\right|_{\phi^\ast_{cl}, \phi_{cl}} ,\nonumber\\
&= \int d^{4}x\,\left.\left\{\partial_{\mu}\phi^\ast(x)\partial^{\mu}\frac{\delta\phi(x)}{\delta \phi(x'')} - m^2\phi^\ast(x)\frac{\delta\phi(x)}{\delta\phi(x'')}\right\}\right|_{\phi_{cl}, \phi^\ast_{cl}},\nonumber\\
&= \int d^{4}x\,\left.\left\{\partial_{\mu}\phi^\ast(x)\partial^{\mu}\delta(x-x'') - m^2\phi^\ast(x)\delta(x-x'')\right\}\right|_{\phi_{cl}, \phi^\ast_{cl}},\nonumber\\
&= \int d^{4}x\,\left.\left\{-\partial_{\mu}\partial^{\mu}\phi^\ast(x) - m^2\phi^\ast(x)\right\}\delta(x-x'')\right|_{\phi_{cl}, \phi^\ast_{cl}}=0.
\end{align}
Again, the expression in the brackets is the Klein-Gordon equation for the conjugate field, which also vanishes for the classical field and, hence, this contribution also vanishes as expected. Finally
\begin{align}
\left.\frac{\delta^{2} S}{\delta \phi^\ast(x')\delta \phi(x'')}\right|_{\phi_{cl}, \phi_{cl}} &= \int d^{4}x\,\left.\frac{\delta^{2} \mathcal{L}}{\delta\phi^\ast(x')\delta \phi(x'')}\right|_{\phi_{cl}, \bar{\phi}_{cl}}  ,\nonumber\\
&= \int d^{4}x\,\left.\left\{\partial_{\mu}\frac{\delta\phi^\ast(x)}{\delta \phi^\ast(x')}\partial^{\mu}\frac{\delta\phi(x)}{\delta \phi(x'')} - m^2\frac{\delta\phi^\ast(x)}{\delta\phi^\ast(x')}\frac{\delta\phi(x)}{\delta\phi(x'')}\right\}\right|_{\phi_{cl}, \phi^\ast_{cl}},\nonumber\\
&= \int d^{4}x\,\left.\left\{\partial_{\mu}\delta(x-x')\partial^{\mu}\delta(x-x'') - m^2\delta(x-x')\delta(x-x'')\right\}\right|_{\phi_{cl}, \phi^\ast_{cl}},\nonumber\\
&= \int d^{4}x\,\left.\left\{-\partial_{\mu}\partial^{\mu}\delta(x-x'') - m^2\delta(x-x'')\right\}\delta(x-x')\right|_{\phi_{cl}, \phi^\ast_{cl}}.
\end{align}
This expression does not vanish and, hence, contributes to the fluctuation in the Noether's current.

The fluctuation can be found by computing, $S_2$,
\begin{align}
S_2 &= \int d^{4}x'\int d^{4}x'' \,\Delta\phi^\ast(x')\Delta\phi(x'')\left.\frac{\delta^{2} S}{\delta \phi^\ast(x')\delta \phi(x'')}\right|_{\phi_{cl}, \phi^\ast_{cl}} ,\nonumber\\
&= \int d^{4}x\int d^{4}x'\int d^{4}x'' \,\Delta\phi^\ast(x')\Delta\phi(x'')\left\{-\partial_{\mu}\partial^{\mu}\delta(x-x'') - m^2\delta(x-x'')\right\}\delta(x-x'),\nonumber\\
&= \int d^{4}x\int d^{4}x'' \,\Delta\phi^\ast(x)\Delta\phi(x'')\left\{-\partial_{\mu}\partial^{\mu}\delta(x-x'') - m^2\delta(x-x'')\right\},\nonumber\\
&= \int d^{4}x\int d^{4}x'' \,\Delta\phi(x'')\left\{-\partial_{\mu}\partial^{\mu}\Delta\phi^\ast(x) - m^2\Delta\phi^\ast(x)\right\}\delta(x-x''),\nonumber\\
&= \int d^{4}x \,\Delta\phi(x)\left\{-\partial_{\mu}\partial^{\mu}\Delta\phi^\ast(x) - m^2\Delta\phi^\ast(x)\right\},\nonumber\\
&= \int d^{4}x \,\left\{\partial_{\mu}\Delta\phi^\ast(x)\partial^{\mu}\Delta\phi(x) - m^2\Delta\phi^\ast(x)\Delta\phi(x)\right\}.
\end{align}
Hence,
\begin{equation}
\mathcal{L}_{2} = \bigg\{\partial_{\mu}\Delta\phi^\ast(x)\partial^{\mu}\Delta\phi(x) - m^2\Delta\phi^\ast(x)\Delta\phi(x)\bigg\}.
\end{equation}

The fluctuation, $F^{\mu}$, in a field $\phi$ is given by
\begin{equation}
\alpha\int d^{4}x\,\partial_{\mu}F^{\mu} = \alpha\int d^{4}x\,\left\{\frac{\partial \mathcal{L}_{2}}{\partial \phi} - \partial_{\mu}\left(\frac{\partial \mathcal{L}_{2}}{\partial (\partial_{\mu}\phi)}\right)\right\}\delta\phi.
\end{equation}
For a spacetime translation one has
\begin{equation}
\alpha = a^{\nu} \qquad\mathrm{and}\qquad \delta\phi = \partial_{\nu}\phi.
\end{equation}
Note that, as we have expanded the field about the classical path, $\phi = \phi_{cl} + \Delta\phi$, which is fixed, the change in the field is given only given by $\Delta\phi$. Hence, 
\begin{equation}
\partial_{\nu}\phi = \partial_{\nu}\Delta\phi \qquad\mathrm{and}\qquad \frac{\partial}{\partial\phi} = \frac{\partial}{\partial\Delta\phi}.
\end{equation}
Thus, we can write
\begin{equation}
\alpha\int d^{4}x\,\partial_{\mu}F^{\mu} = a^{\nu}\int d^{4}x\,\left\{\frac{\partial \mathcal{L}_{2}}{\partial \Delta\phi} - \partial_{\lambda}\left(\frac{\partial \mathcal{L}_{2}}{\partial (\partial_{\lambda}\Delta\phi)}\right)\right\}\partial_{\nu}\Delta\phi .
\end{equation}
In this case, there are two fluctuating fields, the field, $\phi$, and the conjugate field, $\phi^\ast$. The contribution from the field, $\phi$, is
\begin{align}
f_{\phi} &= a^{\nu}\int d^{4}x\,\left\{\frac{\partial \mathcal{L}_{2}}{\partial \Delta\phi} - \partial_{\lambda}\left(\frac{\partial \mathcal{L}_{2}}{\partial (\partial_{\lambda}\Delta\phi)}\right)\right\}\partial_{\nu}\Delta\phi,\nonumber\\
&= a^{\nu}\int d^{4}x\,\bigg\{-m^2\Delta\phi^\ast\frac{\partial \Delta\phi}{\partial \Delta\phi} - \partial_{\lambda}\left(\partial_{\mu}\Delta\phi^\ast\frac{\partial\left[\partial^{\mu}\Delta\phi\right]}{\partial\left[\partial_{\lambda}\Delta\phi\right]}\right) \bigg\}\partial_{\nu}\Delta\phi,\nonumber\\
&= a^{\nu}\int d^{4}x\,\bigg\{-m^2\Delta\phi^\ast\left(\partial_{\nu}\Delta\phi\right) - \left(\partial^{\lambda}\partial_{\lambda}\Delta\phi^\ast\right)\partial_{\nu}\Delta\phi \bigg\},
\end{align}
and the contribution from the conjugate field, $\phi^\ast$, is
\begin{align}
f_{\phi^\ast} &= a^{\nu}\int d^{4}x\,\left\{\frac{\partial \mathcal{L}_{2}}{\partial \Delta\phi^\ast} - \partial_{\lambda}\left(\frac{\partial \mathcal{L}_{2}}{\partial (\partial_{\lambda}\Delta\phi^\ast)}\right)\right\}\partial_{\nu}\Delta\phi^\ast,\nonumber\\
&= a^{\nu}\int d^{4}x\,\bigg\{-m^2\frac{\partial \Delta\phi^\ast}{\partial \Delta\phi^\ast}\Delta\phi - \partial_{\lambda}\left(\frac{\partial\left[\partial_{\mu}\Delta\phi^\ast\right]}{\partial\left[\partial_{\lambda}\Delta\phi^\ast\right]}\right)\partial^{\mu}\Delta\phi \bigg\}\partial_{\nu}\Delta\phi^\ast,\nonumber\\
&= a^{\nu}\int d^{4}x\,\bigg\{-m^2\left(\partial_{\nu}\Delta\phi^\ast\right)\Delta\phi - \left(\partial^{\lambda}\partial_{\lambda}\Delta\phi\right)\partial_{\nu}\Delta\phi^\ast \bigg\}.
\end{align}
Hence, the full fluctuation is
\begin{align}
\alpha\int d^{4}x\,\partial_{\mu}F^{\mu} &= f_{\phi} + f_{\phi^\ast} ,\nonumber\\
&= a^{\nu}\int d^{4}x\,\bigg\{-m^2\Delta\phi^\ast\left(\partial_{\nu}\Delta\phi\right) - \left(\partial^{\lambda}\partial_{\lambda}\Delta\phi^\ast\right)\partial_{\nu}\Delta\phi \bigg\} ,\nonumber\\
&\hspace{2cm} + a^{\nu}\int d^{4}x\,\bigg\{-m^2\left(\partial_{\nu}\Delta\phi^\ast\right)\Delta\phi - \left(\partial^{\lambda}\partial_{\lambda}\Delta\phi\right)\partial_{\nu}\Delta\phi^\ast \bigg\},\nonumber\\
&= a^{\nu}\int d^{4}x\,\bigg\{-\bigg(\left(\partial^{\lambda}\partial_{\lambda}\Delta\phi\right)\partial_{\nu}\Delta\phi^\ast+\left(\partial^{\lambda}\partial_{\lambda}\Delta\phi^\ast\right)\partial_{\nu}\Delta\phi\bigg)-m^2\bigg(\Delta\phi^\ast\left(\partial_{\nu}\Delta\phi\right)+\left(\partial_{\nu}\Delta\phi^\ast\right)\Delta\phi\bigg)\bigg\}.
\label{Dfluc}
\end{align}
One can proceed by noting that the Stress-Energy Tensor for a complex scalar field is give by
\begin{align}
T^{\mu}_{\;\;\nu}(\phi) &= \left(\frac{\partial \mathcal{L}}{\partial (\partial_{\mu}\phi)}\right)\partial_{\nu}\phi+\partial_{\nu}\phi^\ast\left(\frac{\partial \mathcal{L}}{\partial (\partial_{\mu}\phi^\ast)}\right)-\eta^{\mu}_{\;\;\nu}\mathcal{L},\nonumber\\
&=\partial^{\mu}\phi^\ast\partial_{\nu}\phi + \partial_{\nu}\phi^\ast\partial^{\mu}\phi - \eta^{\mu}_{\;\;\nu}\left( \partial_{\lambda}\phi^\ast\partial^{\lambda}\phi - m^2\phi^\ast\phi\right) 
\end{align}
Taking the divergence of the stress energy tensor and relabeling some repeated indices in the second line leads to
\begin{align}
\partial_{\mu}T^{\mu}_{\;\;\nu}(\phi) &= \partial_{\mu}\bigg[\partial^{\mu}\phi^\ast\partial_{\nu}\phi + \partial_{\nu}\phi^\ast\partial^{\mu}\phi - \eta^{\mu}_{\;\;\nu}\left( \partial_{\lambda}\phi^\ast\partial^{\lambda}\phi - m^2\phi^\ast\phi\right) \bigg],\nonumber\\
&= \partial_{\mu}\bigg[\partial^{\mu}\phi^\ast\partial_{\nu}\phi + \partial_{\nu}\phi^\ast\partial^{\mu}\phi\bigg] - \partial_{\nu}\bigg[\partial_{\lambda}\phi^\ast\partial^{\lambda}\phi - m^2\phi^\ast\phi \bigg],\nonumber\\
&= \bigg[\partial_{\mu}\partial^{\mu}\phi^\ast\partial_{\nu}\phi + \partial^{\mu}\phi^\ast\partial_{\mu}\partial_{\nu}\phi + \partial_{\mu}\partial_{\nu}\phi^\ast\partial^{\mu}\phi + \partial_{\nu}\phi^\ast\partial_{\mu}\partial^{\mu}\phi\bigg]\nonumber\\
&\qquad - \bigg[\partial_{\nu}\partial_{\lambda}\phi^\ast\partial^{\lambda}\phi + \partial_{\lambda}\phi^\ast\partial_{\nu}\partial^{\lambda}\phi - m^2\partial_{\nu}\phi^\ast\phi  - m^2\phi^\ast\partial_{\nu}\phi \bigg],\nonumber\\
&= \bigg(\left(\partial_{\mu}\partial^{\mu}\phi\right)\partial_{\nu}\phi^\ast + \left(\partial_{\mu}\partial^{\mu}\phi^\ast\right)\partial_{\nu}\phi\bigg) + m^2\bigg(\phi^\ast\left(\partial_{\nu}\phi\right) + \left(\partial_{\nu}\phi^\ast\right)\phi\bigg),
\label{DdT}
\end{align}
Note that the expression in the brackets in Eq. \eqref{Dfluc} is identical to minus Eq. \eqref{DdT} but with the fields $\phi$ and $\phi^\ast$ replaced with the deviation from the classical field values $\Delta\phi$ and $\Delta\phi^\ast$. Hence, we can write the full fluctuation as
\begin{align}
\alpha\int d^{4}x\,\partial_{\mu}F^{\mu} &= a^{\nu}\int d^{4}x\,\bigg\{-\bigg(\left(\partial^{\lambda}\partial_{\lambda}\Delta\phi\right)\partial_{\nu}\Delta\phi^\ast+\left(\partial^{\lambda}\partial_{\lambda}\Delta\phi^\ast\right)\partial_{\nu}\Delta\phi\bigg)-m^2\bigg(\Delta\phi^\ast\left(\partial_{\nu}\Delta\phi\right)+\left(\partial_{\nu}\Delta\phi^\ast\right)\Delta\phi\bigg)\bigg\},\nonumber\\
&= a^{\nu}\int d^{4}x\,\bigg\{-\partial_{\mu}\left[\partial^{\mu}\Delta\phi^\ast\partial_{\nu}\Delta\phi + \partial_{\nu}\Delta\phi^\ast\partial^{\mu}\Delta\phi - \eta^{\mu}_{\;\;\nu}\left( \partial_{\lambda}\Delta\phi^\ast\partial^{\lambda}\Delta\phi - m^2\Delta\phi^\ast\Delta\phi\right) \right]\bigg\},\nonumber\\
&= a^{\nu}\int d^{4}x\,\bigg\{-\partial_{\mu}\Delta T^{\mu}_{\;\;\nu}(\Delta\phi)\bigg\}.
\end{align}
Thus, we can write
\begin{equation}
\alpha\int d^{4}x\,\partial_{\mu}F^{\mu} = a^{\nu}\int d^{4}x\,\partial_{\mu}\bigg\{-\Delta T^{\mu}_{\;\;\nu}(\Delta\phi)\bigg\}.
\end{equation}
Hence, the fluctuation, $F^{\mu}_{\;\;\nu}$, in the Stress-Energy tensor for a complex scalar field is given by
\begin{equation}
F^{\mu}_{\;\;\nu} = -\Delta T^{\mu}_{\;\;\nu}(\Delta\phi),
\end{equation}
as expected. Note that the function that describes the fluctuations in the Stress-Energy Tensor, $\Delta T^{\mu}_{\;\;\nu}(\Delta\phi)$, is necessarily of the canonical form
\begin{equation}
\Delta T^{\mu}_{\;\;\nu}(\Delta\phi) = \left[\partial^{\mu}\Delta\phi^\ast\partial_{\nu}\Delta\phi + \partial_{\nu}\Delta\phi^\ast\partial^{\mu}\Delta\phi - \eta^{\mu}_{\;\;\nu}\left( \partial_{\lambda}\Delta\phi^\ast\partial^{\lambda}\Delta\phi - m^2\Delta\phi^\ast\Delta\phi\right) \right].
\end{equation}
Any symmetrization that relies on the equations of motion for the classical field would not be valid here as the deviations from the classical field, by definition, do not obey the classical equations of motion.

\section{Applications of Vacuum Fluctuations to the Cosmological Constant and The Vacuum Catastrophe}

To evaluate the average vacuum fluctuations of the Stress-Energy Tensor, $\Delta T^{\mu}_{\;\;\nu}$, one can use the path integral formulism to find the matrix element of the energy fluctuations within a spacetime volume and then average over that volume
\begin{equation}
\Delta T^{\mu}_{\;\;\nu} = \frac{1}{L^4}\int d^4x\, \langle -F^{\mu}_{\;\;\nu} \rangle = \frac{1}{L^4}\int d^4x \,\langle \Delta T^{\mu}_{\;\;\nu}(\Delta\phi) \rangle = \frac{1}{L^4}\int d^4x\,\frac{\displaystyle\int\mathcal{D}\Delta\phi^\ast\int\mathcal{D}\Delta\phi\,\left\{\Delta T^{\mu}_{\;\;\nu}(\Delta\phi) \right\} e^{iS/\hbar}}{\displaystyle\int\mathcal{D}\Delta\phi^\ast\int\mathcal{D}\Delta\phi \,e^{iS/\hbar}}.
\end{equation}
As the denominator is not an explicit function of $x^{\mu}$, one can write
\begin{equation}
\Delta T^{\mu}_{\;\;\nu} = \frac{\displaystyle\frac{1}{L^4}\int\mathcal{D}\Delta\phi^\ast\int\mathcal{D}\Delta\phi\,\int d^4x\left\{\Delta T^{\mu}_{\;\;\nu}(\Delta\phi) \right\} e^{iS/\hbar}}{\displaystyle\int\mathcal{D}\Delta\phi^\ast\int\mathcal{D}\Delta\phi \,e^{iS/\hbar}}.
\label{dE}
\end{equation}
We can evaluate the path integral in the usual way by substituting in the Fourier series expansion for $\Delta\phi$ and $\Delta\phi^\ast$
\begin{gather}
\Delta\phi = \frac{1}{L^4}\sum_{n}a_ne^{-ik_{n,\lambda}x^{\lambda}},\\
\Delta\phi^\ast = \frac{1}{L^4}\sum_{n}a^\ast_n e^{ik_{n,\lambda}x^{\lambda}}.
\end{gather}
Thus, one has for the action
\begin{align}
S &= \int d^4x\, \mathcal{L},\nonumber\\
&= \int d^4x\, \left\{\partial_{\mu}\Delta\phi^\ast\partial^{\mu}\Delta\phi - m^2\Delta\phi^\ast\Delta\phi\right\},\nonumber\\
&= \frac{1}{(L^4)^2}\sum_{n}\sum_{j}a^\ast_na_j\left\{k_{n,\mu}k^{\mu}_{j} - m^2\right\}\int d^4x\, e^{i\left(k_{n,\lambda}-k_{j,\lambda}\right)x^{\lambda}},\nonumber\\
&= \frac{1}{(L^4)^2}\sum_{n}\sum_{j}a^\ast_na_j\left\{k_{n,\mu}k^{\mu}_{j} - m^2\right\}(L^4)\delta_{n,j},\nonumber\\
&= \frac{1}{(L^4)}\sum_{j}a^\ast_ja_j\left\{k_{j,\mu}k^{\mu}_{j} - m^2\right\},\nonumber\\
&= \frac{1}{(L^4)}\sum_{j}a^\ast_ja_j\left\{k^{2}_{j} - m^2\right\},\nonumber
\end{align}
and for the vacuum fluctuation 
\begin{align}
\int d^4x\left\{\Delta T^{\mu}_{\;\;\nu}(\Delta\phi) \right\} &= \int d^4x\, \left\{\partial^{\mu}\Delta\phi^\ast\partial_{\nu}\Delta\phi + \partial_{\nu}\Delta\phi^\ast\partial^{\mu}\Delta\phi - \eta^{\mu}_{\;\;\nu}\left( \partial_{\lambda}\Delta\phi^\ast\partial^{\lambda}\Delta\phi - m^2\Delta\phi^\ast\Delta\phi\right)\right\},\nonumber\\
&= \frac{1}{(L^4)^2}\sum_{n}\sum_{j}a^\ast_na_j\left\{k_{n}^{\mu}k_{j,\nu} + k_{n,\nu}k^{\mu}_{j} - \eta^{\mu}_{\;\;\nu}\left(k_{n,\lambda}k^{\lambda}_{j} - m^2\right)\right\}\int d^4x\, e^{i\left(k_{n,\lambda}-k_{j,\lambda}\right)x^{\lambda}},\nonumber\\
&= \frac{1}{(L^4)^2}\sum_{n}\sum_{j}a^\ast_na_j\left\{k_{n}^{\mu}k_{j,\nu} + k_{n,\nu}k^{\mu}_{j} - \eta^{\mu}_{\;\;\nu}\left(k_{n,\lambda}k^{\lambda}_{j} -m^2\right)\right\}(L^4)\delta_{n,j},\nonumber\\
&= \frac{1}{(L^4)}\sum_{j}a^\ast_ja_j\left\{k_{j}^{\mu}k_{j,\nu} + k_{j,\nu}k^{\mu}_{j} - \eta^{\mu}_{\;\;\nu}\left(k^2_{j} - m^2\right)\right\},\nonumber\\
&= \frac{1}{(L^4)}\sum_{j}a^\ast_ja_j\Delta T^{\mu}_{\;\;\nu}(k_j),
\end{align}
where 
\begin{equation}
\Delta T^{\mu}_{\;\;\nu}(k_j) = \left\{k_{j}^{\mu}k_{j,\nu} + k_{j,\nu}k^{\mu}_{j} - \eta^{\mu}_{\;\;\nu}\left(k^2_{j} - m^2\right)\right\}.
\end{equation}
\newpage

One can evaluate the path integrals by substituting these expressions back into Eq. \eqref{dE} and changing variables to the Fourier coefficients. The denominator becomes
\begin{align}
\int\mathcal{D}\Delta\phi^\ast\int\mathcal{D}\Delta\phi\,e^{iS/\hbar} & = e^{iS_{cl}/\hbar}\,C_N J_N \int d\mathrm{Re}[a_1] d\mathrm{Im}[a_1] \cdots \mathrm{Re}[a_{N-1}] d\mathrm{Im}[a_{N-1}]\nonumber\\
&\hspace{4cm}\times e^{\displaystyle\frac{i}{\hbar(L^4)}\sum_{j}(\mathrm{Re}[a_j]^2 + \mathrm{Im}[a_j]^2)\left\{k^{2}_{j} - m^2\right\}},\nonumber\\
& = e^{iS_{cl}/\hbar}\,C_N J_N \prod_{j}\int d\mathrm{Re}[a_j] d\mathrm{Im}[a_j]\,e^{\displaystyle\frac{i}{\hbar(L^4)}(\mathrm{Re}[a_j]^2 + \mathrm{Im}[a_j]^2)\left\{k^{2}_{j} - m^2\right\}},\nonumber\\
& = e^{iS_{cl}/\hbar}\,C_N J_N \prod_{j}\int d\mathrm{Re}[a_j]\,e^{\displaystyle\frac{i}{\hbar(L^4)}\left\{k^{2}_{j} - m^2\right\}\mathrm{Re}[a_j]^2}\nonumber\\
&\hspace{4cm}\times \int d\mathrm{Im}[a_j]\,e^{\displaystyle\frac{i}{\hbar(L^4)}\left\{k^{2}_{j} - m^2\right\}\mathrm{Im}[a_j]^2},
\end{align}
where $J_N$ is the Jacobian of the variable change and $C_N$ is the prefactor for the integrals along each path. Evaluating the Gaussian integrals gives
\begin{equation}
\int\mathcal{D}\Delta\phi^\ast\int\mathcal{D}\,e^{iS/\hbar} = e^{iS_{cl}/\hbar}\,C_N J_N \prod_{j}\sqrt{\frac{-i\pi\hbar L^4}{k^{2}_{j} - m^2}}\sqrt{\frac{-i\pi\hbar L^4}{k^{2}_{j} - m^2}}= e^{iS_{cl}/\hbar}\,C_N J_N \prod_{j}\frac{-i\pi\hbar L^4}{\displaystyle k^{2}_{j} - m^2}.
\end{equation}
The numerator becomes
\begin{align}
\displaystyle\frac{1}{L^4}\int\mathcal{D}\Delta\phi^\ast&\int\mathcal{D}\Delta\phi\int d^4x\left\{\Delta T^{\mu}_{\;\;\nu}(\Delta\phi) \right\} e^{iS/\hbar}\nonumber\\
& = e^{iS_{cl}/\hbar}\,C_N J_N \frac{1}{(L^4)}\int d\mathrm{Re}[a_1] d\mathrm{Im}[a_1] \cdots \mathrm{Re}[a_{N-1}] d\mathrm{Im}[a_{N-1}]\nonumber\\
&\hspace{2cm}\times \frac{1}{(L^4)}\sum_{n}(\mathrm{Re}[a_n]^2 + \mathrm{Im}[a_n]^2)\Delta T^{\mu}_{\;\;\nu}(k_n)\,e^{\displaystyle\frac{i}{\hbar(L^4)}\sum_{j}(\mathrm{Re}[a_j]^2 + d\mathrm{Im}[a_j]^2)\left\{k^{2}_{j} - m^2\right\}},\nonumber\\
& = e^{iS_{cl}/\hbar}\,C_N J_N \frac{1}{(L^4)^2} \prod_{j}\int d\mathrm{Re}[a_j] d\mathrm{Im}[a_j]\nonumber\\
&\hspace{2cm}\times \sum_{n}(\mathrm{Re}[a_n]^2 + \mathrm{Im}[a_n]^2)\Delta T^{\mu}_{\;\;\nu}(k_n)\,e^{\displaystyle\frac{i}{\hbar(L^4)}(\mathrm{Re}[a_j]^2 + d\mathrm{Im}[a_j]^2)\left\{k^{2}_{j} - m^2\right\}},\nonumber\\
& = e^{iS_{cl}/\hbar}\,C_N J_N \frac{1}{(L^4)^2}\sum_{n}\Delta T^{\mu}_{\;\;\nu}(k_n)\prod_{j}\int d\mathrm{Re}[a_j] d\mathrm{Im}[a_j]\nonumber\\
&\hspace{2cm}\times (\mathrm{Re}[a_n]^2 + \mathrm{Im}[a_n]^2)\,e^{\displaystyle\frac{i}{\hbar(L^4)}(\mathrm{Re}[a_j]^2 + d\mathrm{Im}[a_j]^2)\left\{k^{2}_{j} - m^2\right\}}.\nonumber\\
\end{align}
Each term in the sum over $n$ consists of a product of $N-2$ Gaussian $I_0$ integrals (when $j\neq n$) and one Gaussian $I_2$ integral (when $j=n$)
\begin{gather}
I_{0} = \int_{-\infty}^{\infty}dx\,e^{-\alpha x^2} = \sqrt{\frac{\pi}{\alpha}},\\
I_{2} = \int_{-\infty}^{\infty}dx\,x^2\,e^{-\alpha x^2} = \frac{1}{2\alpha}\sqrt{\frac{\pi}{\alpha}}.
\end{gather}
Evaluating the Gaussian integrals leads to
\begin{align}
\displaystyle\frac{1}{L^4}\int\mathcal{D}\Delta\phi^\ast\int\mathcal{D}\Delta\phi\int d^4x\left\{\Delta T^{\mu}_{\;\;\nu}(\Delta\phi) \right\}e^{iS/\hbar}& = e^{iS_{cl}/\hbar}\,C_N J_N \frac{1}{(L^4)^2}\sum_{n}\Delta T^{\mu}_{\;\;\nu}(k_n)\prod_{j}\nonumber\\
&\hspace{1cm}\times \left[\frac{-i\hbar L^4}{\displaystyle 2\left(k^{2}_{n} - m^2\right)}\frac{-i\pi\hbar L^4}{\displaystyle k^{2}_{j} - m^2} + \frac{-i\hbar L^4}{\displaystyle  2\left(k^{2}_{n} - m^2\right)}\frac{-i\pi\hbar L^4}{\displaystyle  k^{2}_{j} - m^2}\right],\nonumber\\
& = -\frac{i\hbar}{(L^4)}\sum_{n}\frac{\Delta T^{\mu}_{\;\;\nu}(k_n)}{\displaystyle k^{2}_{n} - m^2}\left[e^{iS_{cl}/\hbar}\,C_N J_N \prod_{j}\frac{-i\pi\hbar L^4}{\displaystyle  k^{2}_{j} - m^2}\right].
\end{align}
The expression in the square brackets in the numerator is exactly the expression for the path integral in the denominator and, hence, this factor in the numerator cancels with the denominator. Thus, we have
\begin{equation}
\Delta T^{\mu}_{\;\;\nu} =  -\frac{i\hbar}{(L^4)}\sum_{n}\frac{\Delta T^{\mu}_{\;\;\nu}(k_n)}{\displaystyle k^{2}_{n} - m^2} = -\frac{i\hbar}{(L^4)}\sum_{n}\frac{\displaystyle \left\{k_{n}^{\mu}k_{n,\nu} + k_{n,\nu}k^{\mu}_{n} - \eta^{\mu}_{\;\;\nu}\left(k^2_{n} -m^2\right)\right\}}{\displaystyle k^{2}_{n} - m^2},\nonumber\\
\end{equation}
Converting the sum to an integral in the usual way 
\begin{equation}
\frac{1}{(L^4)}\sum_{n} \rightarrow \int \frac{d^2k}{(2\pi)^4},
\end{equation}
leads to
\begin{equation}
\Delta T^{\mu}_{\;\;\nu} =  -i\hbar\int \frac{d^2k}{(2\pi)^4}\frac{\displaystyle \left\{2k^{\mu}k_{\nu} - \eta^{\mu}_{\;\;\nu}\left(k^2 - m^2\right)\right\}}{\displaystyle k^{2} - m^2}.
\label{vf}
\end{equation}

The integral in Eq. \eqref{vf} is formally divergent. One can regularize the integral via dimensional regularization using the following standard integrals in $D$ dimensions in the limit that $\varepsilon\rightarrow 0$
\begin{align}
\int d^D k\, \frac{1}{(k^2 - m^2 + i\varepsilon)^a} &= i\pi^{D/2}(-1)^a \frac{\Gamma(a - D/2)}{\Gamma(a)} \frac{1}{m^{2a-D}}, \\
\int d^D k\, \frac{k^2}{(k^2 - m^2 + i\varepsilon)^a} &= i\pi^{D/2}(-1)^{a+1} \frac{\Gamma(a - D/2 - 1)}{2\Gamma(a)} \frac{D}{m^{2a-D-2}},\\
\int d^D k\, \frac{k^\mu k_\nu}{(k^2 - m^2 + i\varepsilon)^a} &= i\pi^{D/2}(-1)^{a+1} \frac{\Gamma(a - D/2 - 1)}{2\Gamma(a)} \frac{\eta^{\mu}_{\;\;\nu}}{m^{2a-D-2}}.
\end{align}
In this case $a=1$ and $D=4$. Strictly speaking these integrals only exist for $a>D/2$ but we can apply analytical continuation to these expressions to obtain a closed form answer. However, even in this case these integrals do not converge and, hence, we evaluate them in dimension $D=4-2\delta$ to extract the singularity (an infinite vacuum energy) leaving the finite contribution. We have
\begin{align}
\int d^D k\, \frac{1}{\displaystyle k^{2} - m^2 + i\varepsilon} &= -i\pi^{2}m^2\cdot\pi^{-\delta}m^{-2\delta}\cdot\Gamma(-1+\delta), \\
\int d^D k\, \frac{k^2}{\displaystyle k^{2} - m^2 + i\varepsilon}  &= i\pi^{2}m^4\cdot\pi^{-\delta}m^{-2\delta}\cdot\left(2-\delta\right)\Gamma(- 2 + \delta), \\
\int d^D k\, \frac{k^\mu k_\nu}{\displaystyle k^{2} - m^2 + i\varepsilon}  &= i\pi^{2}m^4\eta^{\mu}_{\;\;\nu}\cdot\pi^{-\delta}m^{-2\delta}\cdot\frac{1}{2}\Gamma(- 2 + \delta).
\end{align}
Putting these contributions together one obtains
\begin{equation}
\Delta T^{\mu}_{\;\;\nu} =  \frac{\hbar c}{16\pi^2} m^4\eta^{\mu}_{\;\;\nu}\cdot\pi^{-\delta}m^{-2\delta}\cdot\bigg\{\frac{1}{2}\Gamma(- 2 + \delta) - \left(2-\delta\right)\Gamma(- 2 + \delta)-\Gamma(-1+\delta)\bigg\},
\end{equation}
where the factor of $c$ comes from the $k_0$ (energy) integral. The singularities are contained in the Gamma functions hence we can expand the expression in brackets for small $\delta$. This leads to
\begin{equation}
\Delta T^{\mu}_{\;\;\nu} = \frac{\hbar c}{16\pi^2} m^4\eta^{\mu}_{\;\;\nu}\cdot\pi^{-\delta}m^{-2\delta}\cdot\bigg\{\frac{1}{\delta} + \frac{1}{8}\left(3 - 2\gamma\right) + \mathcal{O}\left(\delta\right)\bigg\},
\end{equation}
where $\gamma$ is the Euler-Mascheroni constant. The singularity is contained in the first term, the second term is the finite term and all the higher order terms vanish as $\delta\rightarrow 0$. Thus we obtain for the finite contribution to the vacuum fluctuations as
\begin{equation}
\Delta T^{\mu}_{\;\;\nu} = \frac{\hbar c}{128\pi^2}m^4\left(3 - 2\gamma\right)\eta^{\mu}_{\;\;\nu}.
\end{equation}
Converting back to mass in SI units gives
\begin{equation}
\Delta T^{\mu}_{\;\;\nu} = \frac{c^5}{128\pi^2\hbar^3}\bar{m}^4\left(3 - 2\gamma\right)\eta^{\mu}_{\;\;\nu}.
\end{equation}

The connection to the Cosmological Constant can be made by noting that the Stress-Energy tensor is the source term for gravitational curvature. With the fluctuation in the Stress-Energy tensor, Einstein's equations without a Cosmological Constant become
\begin{equation}
G_{\mu\nu} = \frac{8\pi G}{c^4} \left(T_{\mu\nu} - \Delta T_{\mu\nu}\right),
\end{equation}
where $G_{\mu\nu}$ is the Einstein Tensor and $G$ is Newton's gravitational constant. Rearranging we have
\begin{gather}
G_{\mu\nu} + \frac{8\pi G}{c^4}\Delta T_{\mu\nu} = \frac{8\pi G}{c^4}T_{\mu\nu},\nonumber\\
G_{\mu\nu} + \frac{c G}{16\pi\hbar^3}\bar{m}^4\left(3 - 2\gamma\right)\eta_{\mu\nu} = \frac{8\pi G}{c^4}T_{\mu\nu},
\end{gather}
comparing this result with Einstein's equations with a Cosmological Constant,
\begin{equation}
G_{\mu\nu} + \Lambda \eta_{\mu\nu} = \frac{8\pi G}{c^4}T_{\mu\nu},
\end{equation}
one can find an expression for the Cosmological Constant
\begin{equation}
\Lambda = \frac{c G}{16\pi\hbar^3}\bar{m}^4\left(3 - 2\gamma\right),
\end{equation}
in units of $m^{-2}$.

\end{document}
